# Supplementary material for: Module-wise Adaptive Adversarial Training for End-to-end Autonomous Driving
Source: arXiv:2409.07321 source file (2024-09-11)
Supplement: Supplementary file 1 [file appendix1.tex]

\newpage
\section*{Main Results of Remaining Tasks}

In the main text, only the most important planning results are reported. Here, we report the \tool defense results of UniAD \cite{hu2023planning} and VAD \cite{jiang2023vad} models on other tasks. Our evaluation metrics are consistent with the metrics originally applied in the models. For UniAD, we evaluate tracking performance using Average Multi-Object Tracking Accuracy (AMOTA$\uparrow$) and assess map alignment through Intersection over Union (IOU$\uparrow$) between predicted and ground-truth maps. Motion forecasting precision is measured by Minimum Average Displacement Error (minADE$\downarrow$), while occupancy accuracy is also evaluated using IOU ($\uparrow$). For VAD, we use mAP ($\uparrow$) (mean Average Precision) for detection and mapping, and minADE ($\downarrow$) for motion forecasting like UniAD.

\subsection{Defense results of UniAD.} 

\textbf{White-box Results.} \Tref{tab:uniad-white} shows UniAD's defense results against white-box attacks among multi-object tracking, mapping, motion forecasting, and occupancy prediction. We compare our \tool with four traditional adversarial training methods: FGSM adversarial training (F-AT), PGD-$\ell_1$ ($P_{1}$), PGD-$\ell_2$ ($P_{2}$), PGD-$\ell_\infty$ ($P_{\infty}$) adversarial training. From these experimental results, we can draw the following observations. %\Tref{tab:vad-black-detection}

\ding{182} Overall, the defense results of \tool on the remaining tasks of UniAD exceed the traditional four adversarial training methods, with 9 rows showing the best performance.

\ding{183} The robustness improvement effect of \tool on driving tasks in UniAD varies, among which \tool achieves the best defense towards occupancy. Except for FGSM attack, \tool far exceeds traditional adversarial training on the other tasks, and there is only a slight performance decrease of 2.2\% when there is no attack.

\ding{184} The track module of UniAD exhibits extremely severe vulnerability, with any attack almost causing the track module to completely crash. The defensive capability of \tool against track tasks under white box attacks is flawed, but surprisingly, this does not affect its superior performance on downstream tasks.

\ding{185} \tool exhibits acceptable performance degradation in the clean settings. In both track and map tasks, \tool performs the best among all defense methods. It is the second best in occupancy , only relatively inferior in motion.

% uniad white
\begin{table}[!t]
\centering

\small

\caption{\textbf{UniAD}'s defense results under \textbf{white box} settings. The bold cell in each row represents the best performance of that row.}
\label{tab:uniad-white}

% Multi-object Tracking
\begin{tabular}{@{}c@{}}

\subfloat[Multi-object tracking ($\uparrow$)]{
\label{tab:uniad-white-track}
\resizebox{\linewidth}{!}{
\begin{tabular}{@{}cc|lcccc|c@{}}
\toprule
\textbf{Method}  & Vanilla & F-AT & $P_{1}$ & $P_{2}$ & $P_{\infty}$ & AVG & \toolns(ours)            \\ \midrule
FGSM             & 0.14   & 0.55 & \textbf{0.57}  & 0.56   & \textbf{0.57}        & 0.56 & \cellcolor[HTML]{EFEFEF} 0.09 \\
MI-FGSM          & \textbf{0.07}   &0.06 & 0.04  & 0.04   & 0.01        &  0.04 & \cellcolor[HTML]{EFEFEF} 0.00 \\
PGD-$\ell_1$      & 0.13   & 0.18 & 0.18  & \textbf{0.26}   & 0.15        &  0.19 & \cellcolor[HTML]{EFEFEF} 0.14 \\
PGD-$\ell_2$      & 0.11   & 0.14 & 0.14  & \textbf{0.16}   & \textbf{0.16}        & 0.15  & \cellcolor[HTML]{EFEFEF} 0.10 \\
PGD-$\ell_\infty$ & 0.05   & 0.08 & 0.08  & \textbf{0.10}   & 0.03        & 0.07  & \cellcolor[HTML]{EFEFEF} 0.01 \\
%Black-box        & /       & 0.340 & 0.345  & 0.341   & 0.342        & 0.342 & \cellcolor[HTML]{EFEFEF} \textbf{0.355} \\
Clean            & \textbf{0.58}   & 0.36 & 0.34  & 0.38   & 0.23        & 0.33  & \cellcolor[HTML]{EFEFEF} 0.38 \\ \bottomrule
\end{tabular}
}}
\end{tabular}

\vspace{0.3cm}

% Online mapping
\begin{tabular}{@{}c@{}}
\subfloat[Online Mapping (\%) ($\uparrow$)]{
\label{tab:uniad-white-map}
\resizebox{\linewidth}{!}{
\begin{tabular}{@{}cc|lcccc|c@{}}
\toprule
\textbf{Method}  & Vanilla & F-AT & $P_{1}$ & $P_{2}$ & $P_{\infty}$ & AVG & \toolns(ours)            \\ \midrule
FGSM             & 20.09   & \textbf{22.98} & 22.39  & 22.68   & 22.54        & 22.65 & \cellcolor[HTML]{EFEFEF} 20.37 \\
MI-FGSM          & 18.23   & 18.24 & 17.31  & 17.73   & 17.73        &  17.50 & \cellcolor[HTML]{EFEFEF} \textbf{19.23} \\
PGD-$\ell_1$      & \textbf{21.23}   & 21.01 & 21.01  & 20.49   & 20.64  & 20.63  & \cellcolor[HTML]{EFEFEF} 21.11 \\
PGD-$\ell_2$      & 20.79   & 20.74 & 20.74  & 20.28   & 20.39        &  20.54 & \cellcolor[HTML]{EFEFEF} \textbf{21.06} \\
PGD-$\ell_\infty$ & 18.31   & 18.97 & 18.97  & 18.55   & 18.49        &  19.24 & \cellcolor[HTML]{EFEFEF} \textbf{19.43} \\
%Black-box        & /       & 0.330 & 0.340  & 0.336   & 0.338        & 0.338 & \cellcolor[HTML]{EFEFEF} \textbf{0.344} \\
Clean            & \textbf{23.93}   & 22.56 & 22.24  & 22.40   & 22.46        &  22.42 & \cellcolor[HTML]{EFEFEF} 22.77 \\ \bottomrule
\end{tabular}}}
\end{tabular}

\vspace{0.3cm}

% Motion Forecasting
\begin{tabular}{@{}c@{}}
\subfloat[Motion Forecasting ($\downarrow$)]{
\label{tab:uniad-white-motion}
\resizebox{\linewidth}{!}{
\begin{tabular}{@{}cc|lcccc|c@{}}
\toprule
\textbf{Method}  & Vanilla & F-AT & $P_{1}$ & $P_{2}$ & $P_{\infty}$ & AVG & \toolns(ours)            \\ \midrule
FGSM             & 0.99   & 0.51 & 0.47  & \textbf{0.46}   & 0.57        &  0.50 & \cellcolor[HTML]{EFEFEF} 0.79 \\
MI-FGSM          & 1.44   & 0.93 & 1.23  & 1.16   & 0.87        & 1.05  & \cellcolor[HTML]{EFEFEF} \textbf{0.74} \\
PGD-$\ell_1$      & 1.12   & 0.81 & 0.81  & 0.90   & 0.74  & 0.82  & \cellcolor[HTML]{EFEFEF} 0.241 \\
PGD-$\ell_2$      & 1.15   & 0.83 & 0.83  & 0.93   & 0.76        & 0.84 & \cellcolor[HTML]{EFEFEF} \textbf{0.75} \\
PGD-$\ell_\infty$ & 1.46   & 0.93 & 0.93  & 1.07   & \textbf{0.84}       & 0.94  & \cellcolor[HTML]{EFEFEF} 0.87 \\
%Black-box        & /       & 0.330 & 0.340  & 0.336   & 0.338        & 0.338 & \cellcolor[HTML]{EFEFEF} \textbf{0.344} \\
Clean            & \textbf{0.49}   & 0.51 & 0.46  & 0.46   & 0.58        & 0.50  & \cellcolor[HTML]{EFEFEF} 0.57 \\ \bottomrule
\end{tabular}}}
\end{tabular}

\vspace{0.3cm}

% Occupancy Prediction
\begin{tabular}{@{}c@{}}
\subfloat[Occupancy Prediction (\%) ($\uparrow$)]{
\label{tab:uniad-white-occ}
\resizebox{\linewidth}{!}{
\begin{tabular}{@{}cc|lcccc|c@{}}
\toprule
\textbf{Method}  & Vanilla & F-AT & $P_{1}$ & $P_{2}$ & $P_{\infty}$ & AVG & \toolns(ours)            \\ \midrule
FGSM             & 48.6   & 63.2 & 64.7  & \textbf{64.8}   & 61.6        &  63.6 & \cellcolor[HTML]{EFEFEF} 53.7 \\
MI-FGSM          & 44.0   & 46.3 & 44.7  & 44.9   & 48.8        &  46.2 & \cellcolor[HTML]{EFEFEF} \textbf{52.5} \\
PGD-$\ell_1$      & 49.8   & 49.9 & 49.9  & 48.7   & 52.8  &  50.3 & \cellcolor[HTML]{EFEFEF} \textbf{56.6} \\
PGD-$\ell_2$      & 48.6   & 49.7 & 49.7  & 48.5   & 52.1        & 49.0  & \cellcolor[HTML]{EFEFEF} \textbf{56.7} \\
PGD-$\ell_\infty$ & 44.2   & 47.0 & 47.0  & 46.1   & 49.9        & 47.5  & \cellcolor[HTML]{EFEFEF} \textbf{53.0} \\
%Black-box        & /       & 0.330 & 0.340  & 0.336   & 0.338        & 0.338 & \cellcolor[HTML]{EFEFEF} \textbf{0.344} \\
Clean            & \textbf{65.1}   & 60.6 & 63.0  & 62.4   &  46.6       & 58.2  & \cellcolor[HTML]{EFEFEF} 62.9 \\ \bottomrule
\end{tabular}}}
\end{tabular}

\vspace{0.3cm}

\end{table}

\textbf{Black-box Results.} \Tref{tab:uniad-black} shows UniAD's defense results against black-box attacks among four remaining tasks. We use \enhanced UniAD as the victim models, with three categories of attack models: the vanilla model with the same architecture, the traditionally adversarial-trained model, and the vanilla model with a different architecture. Based on the results, we can draw the following observations.

\ding{182} Under the black box setting, mat also outperforms traditional adversarial training methods, showing the best performance in the face of attacks 6 times, while the other four defense methods only achieve the best performance 3 times in total.

\ding{183} Similar to the results under the white box setting, \tool has the best robustness enhancement effect on map and occupation, outperforming other four traditional adversarial training methods in every black box attack. However, in black box settings, \tool performs better in improving track performance than white box attacks, but performs poorly on the motion module.

\ding{184} Among the three types of black box attacks implemented, the attacks generated by the traditional adversarial training model architecture pose the strongest threat to the model compared to the other two types of attacks.

% uniad black
\begin{table}[t]
\centering

\small
\caption{\textbf{UniAD}'s defense results under \textbf{black box} settings. The bold cell in each row represents the best performance of that row.}
\label{tab:uniad-black}
% Multi-object Tracking
\begin{tabular}{@{}c@{}}
\subfloat[Multi-object tracking ($\uparrow$)]{
\label{tab:uniad-black-track}
\resizebox{\linewidth}{!}{
\begin{tabular}{@{}cc|lcccc|c@{}}
\toprule
\textbf{Att. Gen.}  & Vanilla & F-AT & $P_{1}$ & $P_{2}$ & $P_{\infty}$ & AVG & \toolns(ours)            \\ \midrule
Vanilla             & 0.21 & 0.09 & 0.07 & 0.15 & 0.07 & 0.09 & \cellcolor[HTML]{EFEFEF} \textbf{0.24} \\
Trad. AT            & 0.12 & 0.12 & \textbf{0.15} & 0.14 & 0.07 & 0.12 & \cellcolor[HTML]{EFEFEF} 0.04 \\
VAD                 & \textbf{0.14} & 0.12 & 0.07 & 0.08 & 0.05 & 0.08 & \cellcolor[HTML]{EFEFEF} 0.02 \\
 \bottomrule
\end{tabular}
}}
\end{tabular}

\vspace{0.3cm}

% Online mapping
\begin{tabular}{@{}c@{}}
\subfloat[Online Mapping (\%) ($\uparrow$)]{
\label{tab:uniad-black-map}
\resizebox{\linewidth}{!}{
\begin{tabular}{@{}cc|lcccc|c@{}}
\toprule
\textbf{Att. Gen.}  & Vanilla & F-AT & $P_{1}$ & $P_{2}$ & $P_{\infty}$ & AVG & \toolns(ours)            \\ \midrule
Vanilla             & 19.69 & 18.99 & 18.01 & 18.38 & 18.54 & 18.48 & \cellcolor[HTML]{EFEFEF} \textbf{21.29} \\
Trad. AT            & 19.05 & 19.15 & 18.16 & 18.19 & 18.74 & 18.56 & \cellcolor[HTML]{EFEFEF} \textbf{19.70} \\
VAD                 & 18.94 & 18.89 & 18.08 & 18.39 & 18.56 & 18.48 & \cellcolor[HTML]{EFEFEF} \textbf{19.77} \\
 \bottomrule
\end{tabular}
}}
\end{tabular}

\vspace{0.3cm}

% Motion Forecasting
\begin{tabular}{@{}c@{}}
\subfloat[Motion Forecasting ($\downarrow$)]{
\label{tab:uniad-black-motion}
\resizebox{\linewidth}{!}{
\begin{tabular}{@{}cc|lcccc|c@{}}
\toprule
\textbf{Att. Gen.}  & Vanilla & F-AT & $P_{1}$ & $P_{2}$ & $P_{\infty}$ & AVG & \toolns(ours)            \\ \midrule
Vanilla             & \textbf{0.67} & 0.93 & 1.15 & 1.08 & 0.82 & 1.00 & \cellcolor[HTML]{EFEFEF} 0.68 \\
Trad. AT            & 1.30 & 0.91 & 1.18 & 1.16 & \textbf{0.82} & 1.02 & \cellcolor[HTML]{EFEFEF} 0.84 \\
VAD                 & 1.29 & 0.92 & 1.18 & 1.04 & \textbf{0.83} & 0.99 & \cellcolor[HTML]{EFEFEF} 0.84 \\
 \bottomrule
\end{tabular}
}}
\end{tabular}

\vspace{0.3cm}

% Occupancy Prediction
\begin{tabular}{@{}c@{}}
\subfloat[Occupancy Prediction (\%) ($\uparrow$)]{
\label{tab:uniad-black-occ}
\resizebox{\linewidth}{!}{
\begin{tabular}{@{}cc|lcccc|c@{}}
\toprule
\textbf{Att. Gen.}  & Vanilla & F-AT & $P_{1}$ & $P_{2}$ & $P_{\infty}$ & AVG & \toolns(ours)            \\ \midrule
Vanilla             & \textbf{61.3} & 47.1 & 45.6 & 45.8 & 49.7 & 47.1 & \cellcolor[HTML]{EFEFEF} 60.0 \\
Trad. AT            & 45.8 & 45.7 & 47.5 & 46.7 & 38.8 & 44.7 & \cellcolor[HTML]{EFEFEF} \textbf{52.8} \\
VAD                 & 46.3 & 47.4 & 45.4 & 45.8 & 49.7 & 47.1 & \cellcolor[HTML]{EFEFEF} \textbf{52.8} \\
 \bottomrule
\end{tabular}
}}
\end{tabular}

\vspace{0.3cm}

\end{table}

\subsection{Defense results of VAD.} 

\textbf{White-box Results.} \Tref{tab:vad-white} shows VAD's defense results against white-box attacks among detection mapping, and motion forecasting. We compare our \tool with four traditional adversarial training methods like UniAD. From these experimental results, we can draw the following observations.

\ding{182} \toolns's defense towards VAD in upstream tasks is not as superior as towards UniAD. The difference is that it exhibits excellent defense performance in the first detection task, contrary to the module level defense trend of UniAD.

\ding{183} The motion module of VAD performs abnormally under attack settings, with its Minimum Average Displacement Error even showing a huge leap of orders of magnitude, and multiple instances where adversarial training cannot defend against attacks. Our \tool has achieved a certain degree of defense against $\ell_1$ and $\ell_2$ attacks. We believe this may be related to vulnerabilities in the motion module of the model itself.

\ding{184} Raw performance without any attacks of \tool is fantastic, reaching the level of vanilla model in detection, and surpassing other methods in map and motion modules, which are very close to the vanilla level.

\textbf{Black-box Results.} \Tref{tab:vad-black} shows VAD's defense results against black-box attacks among four remaining tasks. We use \enhanced VAD as the victim models, with three categories of attack models: the vanilla model with the same architecture, the traditionally adversarial-trained model, and the vanilla model with a different architecture. Based on the results, we can draw the following observations.

\ding{182} Similar to the white box results, \tool exhibits excellent defense and robustness enhancement in detection, but has shortcomings in the map and motion modules.

\ding{183} Relatively weak black box attacks also cause significant anomalies in the motion module, but this does not result in anomalies in the plan task (as shown in the main experiments). We believe that there may be potential loophole in the motion module of the model that do not flow into downstream tasks.

\ding{184} The black box attack generated by the enhanced model has the strongest attack to VAD for all three tasks, while the attack generated by UniAD has the weakest effect.

% vad white
\begin{table}[t]
\centering

\small
\caption{\textbf{VAD}'s defense results under \textbf{white box} settings. The bold cell in each row represents the best performance of that row.}
\label{tab:vad-white}
% Detection
\begin{tabular}{@{}c@{}}
\subfloat[Detection ($\uparrow$)]{
\label{tab:vad-white-detection}
\resizebox{\linewidth}{!}{
\begin{tabular}{@{}cc|lcccc|c@{}}
\toprule
\textbf{Method}  & Vanilla & F-AT & $P_{1}$ & $P_{2}$ & $P_{\infty}$ & AVG & \toolns(ours)            \\ \midrule
FGSM               & 0.07 & 0.07 & \textbf{0.08} & 0.07 & \textbf{0.08} & 0.07 & \cellcolor[HTML]{EFEFEF} \textbf{0.08} \\
MI-FGSM            & 0.11 & 0.09 & 0.10 & 0.11 & 0.10 & 0.10 & \cellcolor[HTML]{EFEFEF} \textbf{0.13} \\
PGD-$\ell_1$       & \textbf{0.12} & 0.10 & 0.11 & 0.11 & 0.10 & 0.10 & \cellcolor[HTML]{EFEFEF} \textbf{0.12} \\
PGD-$\ell_2$       & 0.11 & 0.11 & 0.11 & 0.11 & 0.10 & 0.11 & \cellcolor[HTML]{EFEFEF} \textbf{0.13} \\
PGD-$\ell_\infty$  & 0.10 & 0.10 & 0.10 & \textbf{0.11} & 0.10 & 0.10 & \cellcolor[HTML]{EFEFEF} \textbf{0.11} \\
Clean              & \textbf{0.27} & 0.22 & 0.23 & 0.22 & 0.22 & 0.22 & \cellcolor[HTML]{EFEFEF} \textbf{0.27} \\ \bottomrule
\end{tabular}
}}
\end{tabular}

\vspace{0.3cm}

% Online mapping
\begin{tabular}{@{}c@{}}
\subfloat[Online mapping ($\uparrow$)]{
\label{tab:vad-white-motion}
\resizebox{\linewidth}{!}{
\begin{tabular}{@{}cc|lcccc|c@{}}
\toprule
\textbf{Method}  & Vanilla & F-AT & $P_{1}$ & $P_{2}$ & $P_{\infty}$ & AVG & \toolns(ours)            \\ \midrule
FGSM               & 0.20 & 0.18 & \textbf{0.14} & 0.18 & 0.17 & 0.17 & \cellcolor[HTML]{EFEFEF} 0.41 \\
MI-FGSM            & 0.51 & \textbf{0.43} & 0.48 & 0.46 & 0.45 & 0.46 & \cellcolor[HTML]{EFEFEF} 0.59 \\
PGD-$\ell_1$       & 0.54 & \textbf{0.47} & 0.52 & 0.51 & 0.49 & 0.50 & \cellcolor[HTML]{EFEFEF} 0.58 \\
PGD-$\ell_2$       & 0.53 & 0.50 & 0.52 & 0.50 & \textbf{0.49}& 0.50 & \cellcolor[HTML]{EFEFEF} 0.59 \\
PGD-$\ell_\infty$  & 0.52 & \textbf{0.43} & 0.49 & 0.46 & 0.45 & 0.46 & \cellcolor[HTML]{EFEFEF} 0.60 \\
Clean              & \textbf{0.70} & 0.56 & 0.61 & 0.60 & 0.59 & 0.59 & \cellcolor[HTML]{EFEFEF} 0.64 \\ \bottomrule
\end{tabular}}}
\end{tabular}

\vspace{0.3cm}

% Motion Forecasting
\begin{tabular}{@{}c@{}}
\subfloat[Motion Forecasting ($\downarrow$)]{
\label{tab:vad-white-map}
\huge
\resizebox{\linewidth}{!}{
\begin{tabular}{@{}cc|lcccc|c@{}}
\toprule[2.2pt]
\textbf{Method}  & Vanilla & F-AT & $P_{1}$ & $P_{2}$ & $P_{\infty}$ & AVG & \toolns(ours)            \\ \midrule
FGSM               & 17552.96 & \textbf{9519.38} & 35803.48 & 44512.75 & 18098.47 & 26983.52 & \cellcolor[HTML]{EFEFEF} 16309.52 \\
MI-FGSM            & \textbf{7869.77}  & 8653.98 & 16499.73 & 32943.96 & 16836.45 & 18733.53 & \cellcolor[HTML]{EFEFEF} 14977.09 \\
PGD-$\ell_1$       & 15639.54 & 8519.92 & 24423.64 & 32511.19 & 16666.39 & 20530.29 & \cellcolor[HTML]{EFEFEF} \textbf{7844.80} \\
PGD-$\ell_2$       & 8250.12  & 32404.79 & 24463.88 & 32404.79 & 16499.73 & 26443.30 & \cellcolor[HTML]{EFEFEF} \textbf{0.51} \\
PGD-$\ell_\infty$  & \textbf{8141.57}  & 8684.34 & 16527.27 & 33276.17 & 16922.79 & 18852.64 & \cellcolor[HTML]{EFEFEF} 22916.02 \\
Clean              & \textbf{0.47}     & 0.50    & 0.52     & 0.51     & 0.53     & 0.51     & \cellcolor[HTML]{EFEFEF} 0.49 \\ \bottomrule[2.2pt]
\end{tabular}}}
\end{tabular}

\end{table}

% vad black
\begin{table}[t]
\centering

% \small
\caption{\textbf{VAD}'s defense results under \textbf{black box} settings. The bold cell in each row represents the best performance of that row.}
\label{tab:vad-black}
% Detection
\begin{tabular}{@{}c@{}}
\subfloat[Detection ($\uparrow$)]{
\label{tab:vad-black-detection}
\resizebox{\linewidth}{!}{
\begin{tabular}{@{}cc|lcccc|c@{}}
\toprule
\textbf{Att. Gen.}  & Vanilla & F-AT & $P_{1}$ & $P_{2}$ & $P_{\infty}$ & AVG & \toolns(ours)            \\ \midrule
Vanilla             & 0.12 & 0.10 & 0.10 & 0.10 & 0.10 & 0.10 & \cellcolor[HTML]{EFEFEF} \textbf{0.15} \\
Trad. AT            & 0.10 & 0.10 & 0.09 & 0.10 & 0.09 & 0.09 & \cellcolor[HTML]{EFEFEF} \textbf{0.12} \\
UniAD               & 0.15 & 0.12 & 0.13 & 0.12 & 0.12 & 0.12 & \cellcolor[HTML]{EFEFEF} \textbf{0.16} \\
 \bottomrule
\end{tabular}
}}
\end{tabular}

\vspace{0.3cm}

% Online mapping
\begin{tabular}{@{}c@{}}
\subfloat[Online mapping ($\uparrow$)]{
\label{tab:vad-black-motion}
\resizebox{\linewidth}{!}{
\begin{tabular}{@{}cc|lcccc|c@{}}
\toprule
\textbf{Att. Gen.}  & Vanilla & F-AT & $P_{1}$ & $P_{2}$ & $P_{\infty}$ & AVG & \toolns(ours)            \\ \midrule
Vanilla             & \textbf{0.46} & 0.47 & \textbf{0.46} & \textbf{0.46} & \textbf{0.46} & 0.46 & \cellcolor[HTML]{EFEFEF} 0.67 \\
Trad. AT            & 0.42 & 0.39 & 0.40 & 0.38 & \textbf{0.35} & 0.38 & \cellcolor[HTML]{EFEFEF} 0.58 \\
UniAD               & 0.70 & \textbf{0.56} & 0.61 & 0.60 & 0.59 & 0.59 & \cellcolor[HTML]{EFEFEF} 0.71 \\
 \bottomrule
\end{tabular}
}}
\end{tabular}

\vspace{0.3cm}

% Motion Forecasting
\begin{tabular}{@{}c@{}}
% \huge
\subfloat[Motion Forecasting ($\downarrow$)]{
\label{tab:vad-black-map}
\resizebox{\linewidth}{!}{
\begin{tabular}{@{}cc|lcccc|c@{}}
\toprule
\textbf{Att. Gen.}  & Vanilla & F-AT & $P_{1}$ & $P_{2}$ & $P_{\infty}$ & AVG & \toolns(ours)            \\ \midrule
Vanilla             & \textbf{7174.1} & 8361.59 & 23608.25 & 31678.93 & 16123.52 & 19943.07 & \cellcolor[HTML]{EFEFEF} 13524.38 \\
Trad. AT            & 8291.55 & 17068.63 & 24504.25 & 24667.07 & 16666.4 & 20726.59 & \cellcolor[HTML]{EFEFEF} \textbf{0.51} \\
UniAD               & \textbf{0.46} & 0.50 & 7662.66 & 7770.91 & 0.53 & 3858.65 & \cellcolor[HTML]{EFEFEF} 6565.12 \\
\bottomrule
\end{tabular}
}}
\end{tabular}

\end{table}

\tool exhibits varying defense performance for upstream tasks in the models, and similar trends are observed for different tasks under white box and black box settings. Although \toolns's defense performance in a few sub tasks is not satisfactory, it achieves excellent defense and improvement in the final plan (as shown in the main results). We believe that from a holistic perspective, each task in the end-to-end autonomous driving model collaborates, but there may be conflicts in the direction of robustness improvement for different tasks. We can sacrifice the performance of some unimportant modules to promote the ultimate key goal - planning.
